# Supplementary material for: Measuring and mitigating voting access disparities: a study of race and polling locations in Florida and North Carolina
Source: arXiv:2205.14867 source file (2022-05-30)
Supplement: Supplementary file 1 [file appendix.tex]

\section{Proofs}
\subsection{Proof of tightness for Observation
\label{app:tightness}
\ref{ob:fair-approx}}
Consider minimizing the maximum value of \error for two groups $A$ and $B$ in Figure \ref{fig:bound}, using three clusters. Assume $|A| \gg |B|$ and $0 \approx \error_{\opt(A)}(A) \ll \error_{\opt(B)}(B)$. The points in group $A$ could be grouped in two clusters $A_1$ and $A_2$ with close to zero cost as shown in the figure. The points in group $B$ lie on three line segments $B_1$, $B_2$ and $B_3$ where $B_l$ points are placed on $B_1$ and $B_s$ points are placed on each one of the other two and $B_l \geq 4B_s$. We should note that the line segments are all of size $r$ and the points are distributed uniformly on each one. Since we assumed the size of group $A$ is much larger than the size of group $B$, an optimal clustering for $X$ would have $C_1$, $C_2$ and $C_3$ as its centers. Without loss of generality, if we assume all the points on $B_2$ and $B_3$ are closer to $C_3$ than $C_1$ and $C_2$, then the total cost of clustering with $\opt(X)$ for group $B$ is $\frac{B_lr}{8} + 2B_s(\frac{x}{2} + \frac{r}{2})$.
If for $\epsilon > 0$ we have $x = \frac{1}{B_s}(\frac{B_l - 4B_s}{8}r + \epsilon)$, then the optimal clustering for group $B$ would have $C_{f_1}$, $C_{f_2}$ and $C_{f_3}$ as its centers and $\error_{\opt(X)}(B) = \error_{\opt(B)}(B) + \epsilon$. 
In addition, it is easy to see $\opt(B)$ also minimizes the maximum average \error for both groups where this value for each group is $\frac{r}{4}$. In such setting, for a small enough value of $\epsilon$, we see that an \error{}-Fair clustering, provides a solution which is $\frac{|A|+|B|}{|B|}$ times the optimal unconstrained solution.

\begin{figure*}
\centering
\includegraphics[width=\textwidth]{bound.pdf}
\caption
{Minimizing the average \error for group $B$, provides a solution which is $\frac{|A|+|B|}{|B|}$ times the optimal solution.}    
\label{fig:bound}
\end{figure*}
